# Supplementary material for: GraphMatch: Efficient Large-Scale Graph Construction for Structure from Motion
Source: arXiv:1710.01602 source file (2017-10-04)
Supplement: Supplementary file 1 [file AbstractSuppl.tex]

\begin{abstract}
In this document we provide supplementary materials...
\end{abstract}
